# Supplementary material for: Exemplar Guided Unsupervised Image-to-Image Translation with Semantic Consistency
Source: arXiv:1805.11145 source file (2019-03-13)
Supplement: Supplementary file 1 [file 6-supp_new.tex]

\section{Supplementary material}
% \vspace{-0.2cm}
\label{supp}

This supplementary material includes more  experimental results (\S\ref{sec:supp_exp}), as well as 
additional implementation details regarding the network architecture and training (\S\ref{sec:supp_implement}).

%%%%%%%%%%%%%%%%%%%%%%%%%%%%%%%%%%%%%%%%%%%%%%%
\subsection{Extra experiment results}
\label{sec:supp_exp}

\myparagraph{Face gender translation.} 
The Large-scale CelebFaces Attributes (CelebA) dataset~\citep{liu2015faceattributes} is a large-scale face attributes dataset with more than 200K celebrity images. 
We divide the aligned face images into male and female domains, containing 84,434 and 118,165 images respectively. 
We perform face gender translation on this dataset to show how the proposed method can be generalized to tasks with attributes as styles.
From Fig.~\ref{figure:face}, we observe that EGSC-IT can translate the face gender successfully, and most importantly transfer the style of hair, skin and background according to the given exemplar image, unlike MUNIT.
\revision{In addition, we also provide the male$\rightarrow$female face translation results matrix Fig.~\ref{figure:male2female}. We observe that the output image's content is consistent with the source image's and its style is consistent with the target image's. Such observation can reflect how the latent space changes given different input images, \ie the the content latent is only related to source image since the style information is combined in the decoder part through feature mask and AdaIN techniques.}

\myparagraph{Letter-digit translation.}
To further evaluate the generalization ability of our method, we use EMNIST~\citep{cohen2017emnist} for three translation tasks: 1) black-white letter $\leftrightarrow$ colored digit; 2) black-white digit $\leftrightarrow$ colored letter; 3) black-white letter  $\leftrightarrow$ colored letter.
EMNIST dataset, a set of handwritten character digits, has the same image format and dataset structure with MNIST dataset. 
We apply the same process to EMNIST letter images as that for MNIST single-digit images in the main paper. 
As shown in \ref{figure:supp_letter_digit}, our model trained with only single-digit data can successfully generalize to the letter data.

\myparagraph{Single-digit translation.}
For the quantitative comparison, we also report the SSIM socre of style transfer methods in Tab.~\ref{tab:supp_MNIST_BW_ssim}. 
\revision{In addition, the larger size version of the single-digit translation t-SNE embedding visualization as shown in Fig.~\ref{figure:supp_MNIST_tsne_large}.}

\begin{table}[!htbp]
\centering
\footnotesize
\caption{SSIM evaluation for single-digit translation. Higher is better. * Models are trained using MNIST-Single data as EGSC-IT. }
\scalebox{1}{
\begin{tabular*}{14cm}
{@{\extracolsep{\fill}} l c c c c c c c c c }
\toprule 
& AdaIN* & WCT* & CycleGAN & UNIT & MUNIT & EGSC-IT\\
\midrule[0.6pt]	
	A $\rightarrow$ B &0.282\revision{$\pm$0.103}  &0.061\revision{$\pm$0.064} &0.214\revision{$\pm$0.168} & 0.178\revision{$\pm$0.160} &0.463\revision{$\pm$0.094} & \textbf{0.478\revision{$\pm$ 0.090}}\\
    B $\rightarrow$ A &0.188\revision{$\pm$0.118} &0.063\revision{$\pm$0.084} &0.089\revision{$\pm$0.166} &0.074\revision{$\pm$0.158} &0.227\revision{$\pm$0.128} &\textbf{0.232\revision{$\pm$ 0.131}}\\
\bottomrule[1pt]
\end{tabular*}
}
% \vspace{-1mm}
\label{tab:supp_MNIST_BW_ssim}
\end{table}

\myparagraph{Multi-digit translation.}
The setting of this experiment was presented in the main paper.
Here, we provide more details on the results.
As seen in Fig.~\ref{figure:supp_MNIST_multi_BW}, both CycleGAN and UNIT can not translate the foreground and background color accordingly, and the colors in CycleGAN look more ``fake''. 
This is due to the fact that CycleGAN and UNIT only learn a one-to-one mapping. 
These observations are consistent with the SSIM score in Tab.~\ref{tab:MNIST_multi_BW_ssim}, where both CycleGAN and UNIT have much lower SSIM scores. 
Differently, MUNIT can not translate the foreground color with semantic consistency, and the colors look more ``fake''.
These observations are consistent with the visualization of t-SNE embeddings. 
As to the SSIM score, MUNIT seems comparable to ours although visually it is performing worse. 
The probable reason is that MUNIT can mostly translate the background successfully which occupies the majority of the image.

\myparagraph{Street view translation.}
We also provide a larger size version of the results for GTA5 $\leftrightarrow$ BDD translation as shown in Fig.~\ref{figure:supp_street_view}.
\revision{In addition, we also provide the ablation study results in Fig.~\ref{figure:supp_street_view_ablation}. We observe that: 1) removing feature mask will lead to color mismatches or inaccuracies (\eg Fig.~\ref{figure:supp_street_view_ablation}(a) 1st row 3rd col); 2) removing AdaIN will reduce the model to unimodality (\eg all images are translated to a sunny day with blue sky, see Fig.~\ref{figure:supp_street_view_ablation}(a) 4th col) since the output image's style is not guided by the exemplar image; 3) removing perceptual loss will lead to incorrect style (\eg  Fig.~\ref{figure:supp_street_view_ablation}(b) 5th col) and the color will spread even given the feature mask since there is no perceptual feedback during training (\eg  Fig.~\ref{figure:supp_street_view_ablation}(a) 5th col).}

\begin{table}[!htbp]
\centering
\footnotesize
\caption{SSIM evaluation for multi-digit translation. Higher is better.}
\scalebox{0.9}{
\begin{tabular*}{13.5cm}
{@{\extracolsep{\fill}} l c c c c c c c}
\toprule 
& CycleGAN & UNIT & MUNIT & EGSC-IT\\
\midrule[0.6pt]	
	A $\rightarrow$ B &0.145\revision{$\pm$0.213} &0.239\revision{$\pm$0.256} &0.500\revision{$\pm$0.035} &\textbf{0.503\revision{$\pm$0.035}} \\
    B $\rightarrow$ A &0.130\revision{$\pm$0.216} &0.234\revision{$\pm$0.257} &\textbf{0.501\revision{$\pm$0.036}} &0.495\revision{$\pm$0.036}\\
\bottomrule[1pt]
\end{tabular*}
}
% \vspace{-1mm}
\label{tab:MNIST_multi_BW_ssim}
\end{table}

%%%%%%%%%%%%%%%%%%%%%%%%%%%%%%%%%%%%%%%%%%%%%%%
\subsection{Implementation details}
\label{sec:supp_implement}
%%%%%%%%%%%%%%%%%%%%%%%%%%%%%%%%%%%%%%%%%%%%%%%
The network architecture and training parameters are listed in Tab.~\ref{tab:param}. 
We set the number of down-sampling and up-sampling convolutional layers $n_1=1$ in single-digit translation and $n_1=3$ in other translation experiments. 
Following UNIT~\citep{UNIT}, the number of residual blocks in $Encoder$ and $Generator$ is set to $n_2=4$ with one sharing layer, and the number of convolutional layers in discriminator is set to $n_3=5$. 
The threshold parameter $\eta$ is used to adjust how much the feature mask affects the information flow. Setting $\eta=0$, \ie using the feature maps (paper Fig.~\ref{figure-framework_test} top branch) as feature mask directly, leads to useful information being dropped out and artifacts in the results. Setting $\eta=1$, \ie not using feature mask at all, leads to results without semantic consistency (see paper Fig.~\ref{figure-MNIST_BW}). After experimenting with different values, we fixed it to $0.5$. 
We use the Adam~\cite{Adam} optimizer with $\beta_1=0.5$ and $\beta_2=0.999$. 
The learning rate is polynomially decayed with a power of 0.9, as mentioned in~\citep{chen2018deeplab}. 
In order to keep training stable, we update encoder and generator 5 times, and discriminator 1 time in each iteration.
The loss weights in $\mathcal{L}_\text{UNIT}$ are following~\citep{UNIT}, and $\lambda_c$, $\lambda_s$ are chosen according to the dataset variations and tasks.
For data augmentation, we do left-right flip and random crop. 
In addition, we set a low $\lambda_c$ for face gender translation, since we need to change the shape and add/remove hair in this translation task.

\begin{table}[!htbp]
\centering
\footnotesize
\caption{Network architecture and training parameters.}
\begin{tabular*}{13.5cm}
{@{\extracolsep{\fill}} l c c c c c c c c c}
\toprule 
Translation &$n_1$ &$n_2$ &$n_3$ & Minibatch & Learning rate & $\lambda_s$ & $\lambda_c$ & Iteration  \\
\midrule[0.6pt]	
	Single-digit &1 &4 &5 &8 &1e-5 &1e3 &1e1 &$\sim$60k \\
    Multi-digit &3 &4 &5 &8 &1e-5 &1e4 &1e2 &$\sim$60k \\
    % GTA5$\leftrightarrow$Cityscapes &3 &4 &5 &3 &1e-4 &1e3 &5e2 &$\sim$22k  \\
    GTA5$\leftrightarrow$BDD &3 &4 &5 &3 &1e-4 &1e4 &1e2 &$\sim$22k \\
    Face gender &3 &4 &5 &8 &1e-4 &5e3 &1e1 &$\sim$30k \\
\bottomrule[1pt]
\end{tabular*}
% \vspace{-1mm}
\label{tab:param}
\end{table}

%%%%%%%%%%%%%%%%%%% Figures %%%%%%%%%%%%%%%%%%%%%
\clearpage

\begin{figure*}[!htbp]
  \centering
  \includegraphics[width=1.0\linewidth]{imgs/celeba_all_5g1d_EGSC2.pdf}\\
  \caption{Face gender translation testing results of EGSC-IT. Best viewed in color.}
\label{figure:face}
% \vspace{-0.5cm}
\end{figure*}

\begin{figure*}[!htbp]
  \centering
  \includegraphics[width=1.0\linewidth]{imgs/Celeba_matrix.pdf}\\
  \caption{\revision{Male$\rightarrow$Female translation testing results of EGSC-IT. Best viewed in color.}}
\label{figure:male2female}
% \vspace{-0.5cm}
\end{figure*}

\begin{figure*}[!htbp]
  \centering
  \includegraphics[width=1.0\linewidth]{imgs/out_of_domain_emnist.pdf}\\
  \caption{Letter-digit translation testing results. Note that, models are trained only with single-digit data.}
\label{figure:supp_letter_digit}
% \vspace{-0.5cm}
\end{figure*}

\begin{figure*}[htb]
  \centering
  \includegraphics[width=1.00\linewidth]{imgs/MNIST_BW_tsne_new_randInit_large.pdf}\\
%   \vspace{-0.1cm}
  \caption{\revision{Single-digit translation t-SNE embedding visualization in larger size. {\color{red}Red dots}: real samples. {\color[rgb]{0.255,0.412,0.882}Blue crosses}: generated samples. Best viewed in color.}}
\label{figure:supp_MNIST_tsne_large}
% \vspace{-0.4cm}
\end{figure*}

\begin{figure*}[!htbp]
  \centering
  \includegraphics[width=1.0\linewidth]{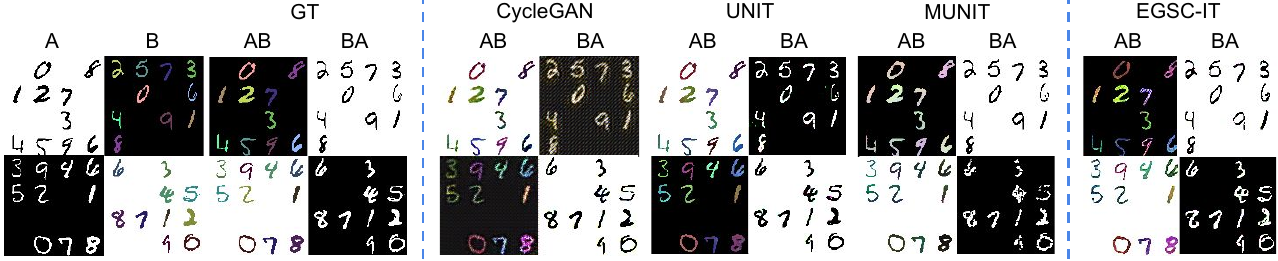}\\
  \caption{Multi-digit translation testing results.}
\label{figure:supp_MNIST_multi_BW}
% \vspace{-0.5cm}
\end{figure*}

\begin{figure*}[!htbp]
  \centering
  \includegraphics[width=1\linewidth]{imgs/MNIST_multi_BW_tsne_new_randInit.pdf}\\
  \caption{\revision{Multi-digit translation t-SNE embedding visualization. {\color{red}Red}: real samples. {\color[rgb]{0.255,0.412,0.882}Blue}: generated samples. Best viewed in color.}}
\label{figure:supp_MNIST_multi_tsne}
% \vspace{-0.5cm}
\end{figure*}

\begin{figure*}
  \centering
  \includegraphics[width=0.8\linewidth]{imgs/street_view_test_result_5g1d_EGSC_large.pdf}\\
  \caption{Street view translation testing results in larger size. Best viewed in color.}
\label{figure:supp_street_view}
% \vspace{-0.5cm}
\end{figure*}

\begin{figure*}
  \centering
  \includegraphics[width=1\linewidth]{imgs/gta2bdd_ablation_paper_v3.pdf}\\
%   GTA$\rightarrow$BDD translation\\
  \caption{\revision{Street view translation ablation study results. Zoom in for more details. Best viewed in color.}}
\label{figure:supp_street_view_ablation}
% \vspace{-0.5cm}
\end{figure*}
